# Supplementary material for: Computer Architecture-Aware Optimisation of DNA Analysis Systems
Source: arXiv:2101.05012 source file (2021-01-13)
Supplement: Supplementary file 1 [file 5.6-server-compare.tex]

\chapter{Appendix: Analysis of Computational Platforms for Nanopore Data Processing}\label{a:rock64-compare}

Processing of the second generation sequencing involves base space data only. Nevertheless they are computationally intensive. Nanopore data processing involves both base space data and the raw signal data. This requirement of raw signal data introduces an additional computational burden. 

The following figure shows a typical nanopore sequencing and analysis workflow.

\begin{itemize}
    \item step 1: sequencing 
    \item step 2: base-calling 
    \item step 3: read alignment (base-space)
    \item step 4: raw signal alignment (e.g., ABEA)
    \item step 5: per-read information extraction  (e.g., methylation calling)
    \item step 6: post-processing (e.g.,variant detection, methylation frequency counting)
\end{itemize}

Post processing refers to genetic/epigenetic variant detection that uses all the reads than span a region.  Thus, this step requires the data for all the reads to be available before processing. However, up to step 4 (including step 4) can be processed on-the-fly. i.e., as reads are being output from the sequencer. 

There are three different approaches to process data up to (including) step 4:

\begin{enumerate}
    \item Wait until the sequencing run completes (48 hours for MinION/GridION and 64 hours for PromethION) and execute the analysis on the full dataset (non real-time).
    \item Process read by read as reads are being output by the sequencer (real real-time).
    \item Process batch by batch as batches of reads become available (near real-time).
\end{enumerate}

For the approach 1, it is a common practise by researchers to execute with all the available CPU-cores on an HPC, intending a fast turn-around time. However, this approach is inefficient due to existing software being unable to efficiently utilise all CPU cores.  

for batch by batch processing, again running with all available threads is unsuitable. 
solutions
write software to be efficient
use MPMT approach
For doing MPMT approach, we do not need an expensive server. A PC cluster or even an ARM SBC cluster may suffice.

To process as fast as possible, a server but a single process multi threaded solution waste CPU resource
on a server with n threads we run for each batch (n threads per each)
minimap2
samtools
nanopolish
we observe that the CPU utilisation is quite low

The workflow/pipeline

nanopolish index
minimap2 - read alignment
samtools sort - sorting alignments by genomic coordinates
samtools index - index for the alignment file
nanopolish call-methylation

Methods tested

Running on the whole dataset at the end of the sequencing run
Running batch by batch

\section{Approach 1: Wait until the sequencing run completes and execute the analysis on the full dataset (non real-time)}

combinations of experiments

Dataset : 778-500ng

data sizes from each tool

Only run on servers as running on distributed systems on the whole dataset at once is not practical. Three cases are tested : 
HDD RAID array
SSD RAID array
NFS mount
PANFS mount (later if needed - not mandotory - problems with quota will come)

ran the workflow with 1,2,4,8,16,32 and 64 threads. Note that multiple threads are for minimap2, samtools sort and nanopolish call-methylation only. Nanopolish index and Samtools index are always run with a single thread as they do not support multithreading.

disk cache was cleared before running each workflow for each number of threads

\subsection{On server with HDD RAID}

Nanopolish index takes the same time for each case as it is run with 1 thread for all the cases. Minimap2 scales well with the number of threads almost linearly upto 32 threads. There is no much improvement from 32 threads to 64 threads but the time had reduced to 0.1 which is an order XXX of for nanopolish (See Table below)

\subsection{On server with SSD RAID}

\subsection{On NFS}

\section{Approach 2: Process batch by batch as batches of reads become available (near real-time)}

combinations of experiments

Datasets 
778-500ng
Systems
	HDD RAID
	SSD RAID
	Distributed
Scheduling
	static
	dynamic - f5pd
Data existence and scratch
	Locally on HDD RAID
	Locally on SSD RAID
	From SSD to RAMDISK
	From HDD to RAMDISK
	From NFS to disk

\subsection{Data already existing on HDD-RAID with static}

\subsection{Data already existing on HDD-RAID with dynamic - f5pd}

SPMT means single process multi threaded - minimap2 and nanopolish methylation calling run with all available 56 threads
MPMP means multi process multi threaded - dataset statically divided into roughly equal 14 partitions. 14 processes run in parallel where each process runs  minimap2 and nanopolish methylation calling with 4 threads
